# Supplementary material for: Efficient Query Repair for Aggregate Constraints
Source: arXiv:2511.00826 source file (2025-11-02)
Supplement: Supplementary file 1 [file appendix.tex]

\section{Example Use Cases}\label{sec:usecases} %Copied from TapP paper

%\BGI{I think one problem we have with the current structure is that we already walk through a relatively detailed fairness example in the intro making this section partially redundant. One option could be to merge this example intro and align it with Figure 1.}

% We describe two use cases to highlight the need for repairing user queries to fulfill aggregate constraints on the query's result.

%%%%%%%%%%%%%%%%%%%%%%%%%%%%%%%%%%%%%%%%%%%%%%%%%%%%%%%%%%%%%%%%%%%%%%%%%%%%%%%%

%%%%%%%%%%%%%%%%%%%%%%%%%%%%%%%%%%%%%%%%%%%%%%%%%%%%%%%%%%%%%%%%%%%%%%%%%%%%%%%%
\subsection{Company Product Management}\label{subsec:generalUse}

%Consider a supply and demand scenario over the TPC-H Benchmark schema~\cite{tpc-hLink}.
A retail company aims to monitor product performance by retrieving information about the parts of type “Large Brushed” with a size greater than 10 that are supplied by suppliers located in Europe.\BG{This sounds different from the paragraph after the query which talks about product selection for stock management. We need to align these two.}
%%%%%%%%%%%%%%%%%%%%%%%%%%%%%%%%%%%%%%%%%%%%%%%%%%%%%%%%%%%%%%%%%%%%%%%%%%%%%%%%
The company uses the following query to retrieve this information:

%%%%%%%%%%%%%%%%%%%%%%%%%%%%%%%%%%%%%%%%%%%%%%%%%%%%%%%%%%%%%%%%%%%%%%%%%%%%%%%%
% \mypar{The Query}
\begin{lstlisting}
@\small\upshape\bf\ttfamily{Q2}@: SELECT *
    FROM part, supplier, partsupp, nation, region
    WHERE p_partkey = ps_partkey AND
        s_suppkey = ps_suppkey AND p_size >= 10
        AND s_nationkey = n_nationkey
        AND n_regionkey = r_regionkey
        AND p_type = 'LARGE BRUSHED'
        AND r_name = 'EUROPE'
\end{lstlisting}

%%%%%%%%%%%%%%%%%%%%%%%%%%%%%%%%%%%%%%%%%%%%%%%%%%%%%%%%%%%%%%%%%%%%%%%%%%%%%%%%
%This query is hardcoded in the company's inventory management system, which is maintained by an external vendor. The system is designed to automatically retrieve all relevant product and supplier details, ensuring uniformity in reporting across all company branches. As a result, the manager cannot modify the query logic directly.

The company, however, has set an aggregate constraint to manage its product selection and ensure effective inventory planning. They want to avoid overstocking under-performing products that contribute less to revenue.\BG{This is not reflected in the constraint!}
The constraint requires that products from UK only contribute 10\% to 30\% of the total revenue of the result set in order to minimize supply chain disruptions. Formally, the constraint is defined as follows:
%%%%%%%%%%%%%%%%%%%%%%%%%%%%%%%%%%%%%%%%%%%%%%%%%%%%%%%%%%%%%%%%%%%%%%%%%%%%%%%%
% \vspace{-2mm}
% \[
% 0.3 \leq \frac{\sum \text{Revenue}_{\text{Selected Products}}}{\sum \text{Revenue}_{\text{All Products}}} \leq 0.5
% \]
\[
0.1 \leq \frac{\sum \text{Revenue}_{\text{ProductsSelectedFromUK}}}{\sum \text{Revenue}_{\text{Selected Products}}} \leq 0.3
\]
% Where:

% $\text{Revenue}_{\text{Selected Products}} = \sum (l\_extendedprice \times (1 - l\_discount))$ and $\sum \text{Revenue}_{\text{All Products}} = \sum (l\_extendedprice \times (1 - l\_discount))$ for all products.

Prior work on query repair ~\cite{AlbarrakS17} only supports constraints on a single aggregation result while the constraint shown above is an arithmetic combination of aggregation results as supported in our framework. % , e.g., simplistic average using a single attribute from the dataset.
% In this case, we have a aggregation over multiple attributes.

%%% Local Variables:
%%% mode: LaTeX
%%% TeX-master: "../main"
%%% End:

\section{Comparison with Brute Force} \label{subsec: cpmare with brute force}
%\SLI{Consolidating all the evaluation results into a single section may become overwhelming. Instead, we can divide them into multiple sections: one for the performance evaluation of our methods, one that highlights the key factors influencing our method's performance, and a third for comparing our performance to that of Erica.}

In this section, we compare the brute-force (BF) method with our proposed techniques, FF and RP. In all experiments, we use green for BF, shades of blue for FF, and shades of red for RP. We evaluate the performance of these techniques using the Healthcare dataset with queries Q1 and Q2, as well as constraint C1 with different bounds using our default settings: a dataset size of 50K, 5 branches, top-7 solutions, and a bucket size of 15.

\begin{figure}[htbp]
    \centering
    \begin{subfigure}[t]{1\linewidth}
        \centering
        \includegraphics[width=\linewidth]{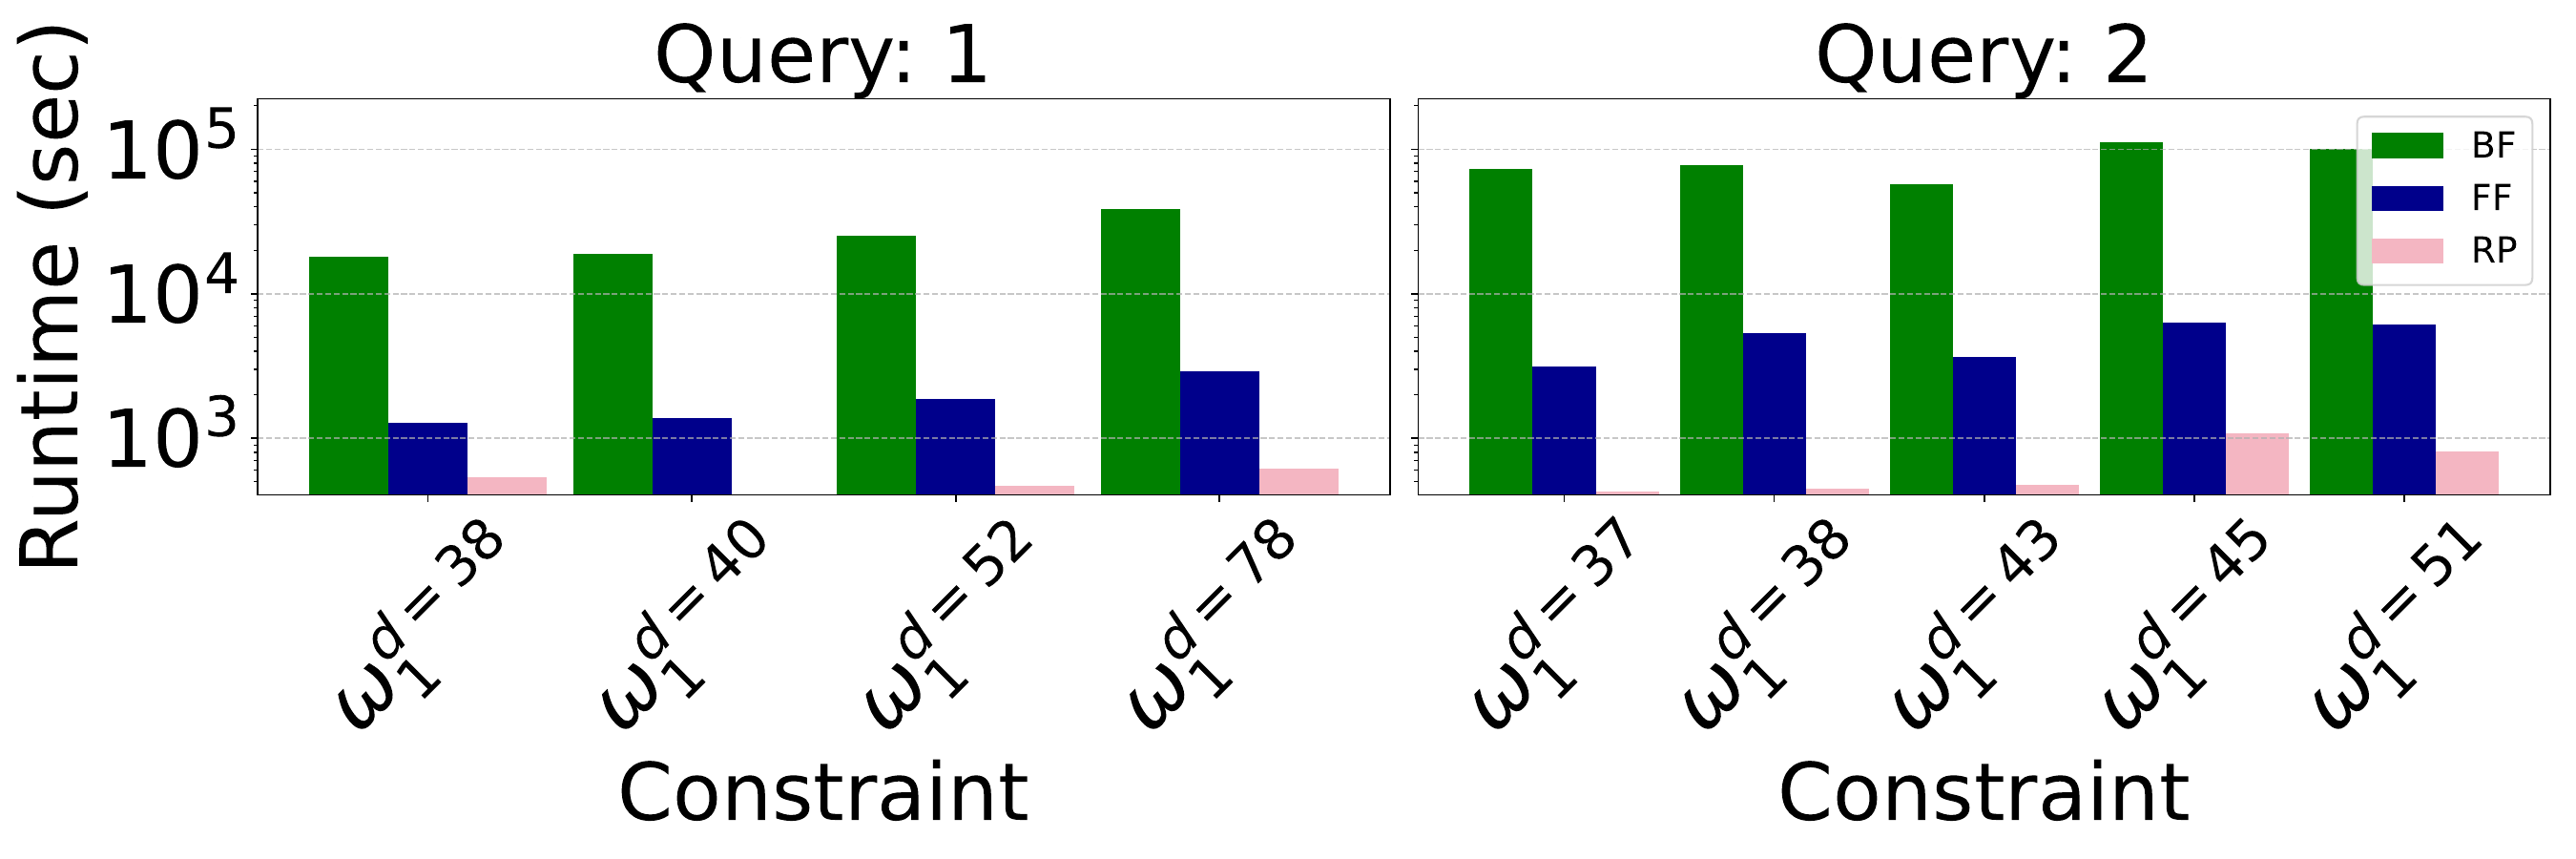}
        \caption{Comparison of Runtime.}
        \label{fig:runtime_comparison}
    \end{subfigure}
    \vspace{0.2cm} % Adjust vertical spacing if needed
    \begin{subfigure}[t]{1\linewidth}
        \centering
        \includegraphics[width=\linewidth]{comparison_fully_vs_ranges_bruteforce_Checked Num.pdf}
        \caption{Comparison of the number of Candidate solutions evaluated.}
        \label{fig:checked_comparison}
    \end{subfigure}
    \vspace{0.2cm} % Adjust vertical spacing if needed
    \begin{subfigure}[t]{1\linewidth}
        \centering
        \includegraphics[width=\linewidth]{comparison_fully_vs_ranges_bruteforce_Access Num.pdf}
        \caption{Comparision of number of clusters accessed.}
        \label{fig:access_comparison}
    \end{subfigure}
    \caption{Comparison of runtime, number candidate solutions evaluated, and number of clusters accessed for Healthcare dataset.}
    \label{fig:comparison_combined}
    % \SLI{Shorten y-axis label, e.g., Number of Candidate Solutions Checked to NCSC, and increase the font size of y-axis.}
\end{figure}

\mypar{Performance}
Figure~\ref{fig:runtime_comparison} illustrates the runtime of the three algorithms \textbf{BF, FF, and RP} for queries Q1 and Q2 across constraint C1 with different bounds.
% \SLI{What are the constraints from C1 to C6? What are the meaning of them? Eventually, the constraints in Table 3 should be explained.}
The BF algorithm consistently exhibits the highest runtime, as it processes all data points for each repair and exhaustively evaluates all combinations, leading to significant computational overhead. Consequently, as shown in Figure~\ref{fig:access_comparison}, BF also incurs the highest number of accesses, as it scans every individual data point in the dataset. The FF algorithm substantially reduces runtime by employing an optimized traversal technique that filters data based on the bounds of the clustering tree. Instead of accessing each data point, FF only accesses cluster boundaries, as demonstrated in Figure~\ref{fig:access_comparison}, where it reduces the number of accesses. The RP algorithm further improves performance by efficiently pruning irrelevant repair combinations using range-based constraints. As observed in Figure~\ref{fig:access_comparison}, RP significantly minimizes the number of accesses to clusters, making it the most efficient approach.
%For instance, under constraint C1B5, the runtime of the BF algorithm exceeds 38,000 seconds, whereas FF and RP complete execution in approximately 2,900 seconds and 620 seconds, respectively. This result highlights that 
In general, FF outperforms BF by at least an order of magnitude, while RP achieves an additional fivefold improvement, showcasing the efficiency of the proposed approaches.

\mypar{Number of Candidate Repairs}
The number of candidate repairs is calculated as the product of the unique possible values for all predicates. For ACSIncome dataset, this number ranges from approximately 14K to 18K. In Healthcare dataset, it varies between approximately 10K and 22K. For TPCH queries, the number of possible repair candidates is approximately 38K.

\mypar{Number of Candidate Solutions Checked}
Figure~\ref{fig:checked_comparison} illustrates the number of candidate solutions evaluated by each algorithm for query Q1 and Q2 across different bounds of C1. The BBF and FF methods exhibit identical counts, as both exhaustively examine all possible repairs. In contrast, the RP method achieves the lowest number due to its efficient use of ranges. For example, under constraint C1B5, the BBF and FF methods evaluate over 7,400 constraints, as they individually assess each possible candidate repair. Meanwhile, the RP method evaluates approximately 850 candidate repair by leveraging ranges to skip sets of unpromising repairs. This reduction highlights the efficiency of the RP technique in eliminating redundant evaluations and minimizing computational overhead.
Based on the results of the experiment, it is clear that the BF algorithm performs considerably worse than our proposed algorithms in terms of runtime. Given its poor performance and impracticality for real-world use cases, we have decided to exclude the BF algorithm from the remaining experiments. Instead, we will focus on comparing the FF and RP algorithms, as they represent more realistic and competitive solutions.

%%%%%%%%%%%%%%%%%%%%%%%%%%%%%%%%%%%%%%%%%%%%%%%%%%%%%%%%%%%%%%%%%%%%%%%%%%%%%%%%

\begin{table*}[htbp] % Use table* to span both columns
    \caption{Constraints for Experimentation}
    \label{tab:constraints-full}
    \centering
    \begin{tabular}{|p{2cm}|p{8.5cm}|p{6cm}|p{1.2cm}|}
    \hline
    \textbf{Constraint ID} & \textbf{Expression} & \textbf{Bounds} \\ \hline
    C1 &
    $B_l \leq \frac{\text{count}(\text{race} = 1 \land \text{label} = 1)}{\text{count}(\text{race} = 1)} - \frac{\text{count}(\text{race} = 2 \land \text{label} = 1)}{\text{count}(\text{race} = 2)} \leq B_u$ &
    $B_1$:[0.44, 0.5], $B_2$:[0.25, 0.5], $B_3$:[0.42, 0.5], $B_4$:[0.35, 0.5], $B_5$:[0.5, 0.6], $B_6$:[0.23, 0.25], $B_7$:[0.25, 0.4], $B_8$:[0.34, 0.39], $B_9$:[0.2, 0.25], $B_{10}$:[0.3, 0.5], $B_{11}$: [0.31, 0.36], $B_{12}$: [0.2, 0.5]
    \\ \hline
    C2 &
    $B_l \leq \frac{\text{count}(\text{ageGroup} = 1 \land \text{label} = 1)}{\text{count}(\text{ageGroup} = 1)} - \frac{\text{count}(\text{ageGroup} = 2 \land \text{label} = 1)}{\text{count}(\text{ageGroup} = 2)} \leq B_u$ & $B_1$:[0.44, 0.5], $B_2$:[0.25, 0.5], $B_3$:[0.42, 0.5], $B_4$:[0.35, 0.5], $B_5$:[0.5, 0.6]
    \\ \hline
    C3 &
    $B_l \leq \frac{\text{count}(\text{sex} = 1 \land \text{PINCP} \geq 20k)}{\text{count}(\text{sex} = 1)} - \frac{\text{count}(\text{sex} = 2 \land \text{PINCP} \geq 20k)}{\text{count}(\text{sex} = 2)} \leq B_u$ &  $B_1$:[0.34, 0.39], $B_2$:[0.3, 0.5], $B_3$:[0.44, 0.5], $B_4$:[0.25, 0.5], $B_5$:[0.2, 0.25], $B_6$:[0.15, 0.4], $B_7$:[0.23, 0.25], $B_8$:[0.22, 0.4], $B_9$:[0.34, 0.36], $B_{10}$:[0.34, 0.35], $B_{11}$:[0.35, 0.36], $B_{12}$:[0.39, 0.4], $B_{13}$:[0.42, 0.44]
    \\ \hline
    C4 &
    $B_l \leq \frac{\text{count}(\text{RACE} = 1 \land \text{PINCP} \geq 15k)}{\text{count}(\text{RACE} = 1)} - \frac{\text{count}(\text{RACE} = 2 \land \text{PINCP} \geq 15k)}{\text{count}(\text{RACE} = 2)} \leq B_u$ & $B_1$:[0.34, 0.39], $B_2$:[0.3, 0.5], $B_3$:[0.44, 0.5], $B_4$:[0.25, 0.5], $B_5$:[0.2, 0.25], $B_6$:[0.37, 0.39], $B_7$:[0.38, 0.39], $B_8$:[0.34, 0.35], $B_9$:[0.34, 0.39], $B_{10}$:[0.3, 0.5], $B_{11}$:[0.23, 0.25], $B_{12}$:[0.34, 0.36], $B_{13}$:[0.3, 0.33], $B_{14}$:[0.32, 0.35]
    \\ \hline
    C5 &
    $B_l \leq \frac{\text{sum}(\text{p\_retailprice})}{\text{count}(\text{p\_retailprice})} - \frac{\text{sum}(\text{s\_acctbal})}{\text{count}(\text{s\_acctbal})}$ & $B_1$: 0.0014, $B_2$: 0.0025, $B_3$: 0.005, $B_4$: 0.01, $B_5$: 0.026
    \\ \hline
     C6 Erica~\cite{LM23}&
    $\{\text{count}(\text{race}) = \text{race1}\} \leq B_u, \{\text{count}(\text{age}) = \text{group1}\} \leq B_u$ & \{300, 170\}
    \\ \hline
     C7 Erica~\cite{LM23}&
    $\{\text{count}(\text{race}) = \text{race1}\} \leq B_u,\{\text{count}(\text{age}) = \text{group1}\} \leq B_u, \newline\{\text{count}(\text{age}) = \text{group3}\} \leq B_u$  & \{300, 170,250\}
    \\ \hline
    C8 Erica~\cite{LM23}&
$\{\text{count}(\text{Sex}) = \text{Female}\} \leq B,$
$\{\text{count}(\text{Race}) = \text{Black}\} \leq B,$
$\{\text{count}(\text{Marital}) = \text{Divorced}\} \leq B$ &
$\text{B1}=\{30, 150, 10\}, \quad \text{B2} = \{30, 300, 25\},$
$\text{B3} = \{10, 650, 50\}, \quad \text{B4} = \{15, 200, 15\}$
     \\ \hline
    \end{tabular}
\end{table*}

% %%%%%%%%%%%%%%%%%%%%%%%%%%%%%%%%%
% \begin{table*}
%     \caption{Queries for Experimentation}
%     \label{tab:queries}
%     \centering
%     \adjustbox{max width=\columnwidth}{
%     \begin{tabular}{|c|c|p{7cm}|p{1.5cm}|}
%     \hline
%          \textbf{Dataset} & \textbf{ID} & \textbf{Query} & \textbf{Source} \\\hline
%          \multirow{3}{*}{Healthcare}
%          & Q1 & \lstset{aboveskip=0pt, belowskip=0pt}\begin{lstlisting}[language=Python]
% SELECT * FROM Healthcare
% WHERE income >= 200K and
% num-children >= 3 and county <= 3
% \end{lstlisting} & Erica~\cite{LM23} \\ \cline{2-4}
%   & Q2 & \lstset{aboveskip=0pt, belowskip=0pt}\begin{lstlisting}[language=Python]
% SELECT * FROM Healthcare
% WHERE income <= 100K and
% complications >= 5 and num-children >= 4
% \end{lstlisting} & Erica~\cite{LM23} \\ \cline{2-4}
%   & Q3 & \lstset{aboveskip=0pt, belowskip=0pt}\begin{lstlisting}[language=Python]
% SELECT * FROM Healthcare
% WHERE income >= 300K and
% complications >= 5 and county == 1
% \end{lstlisting} & Generated \\ \hline

%          \multirow{3}{*}{Adult-CI} & Q4 &
%          \lstset{aboveskip=0pt, belowskip=0pt}\begin{lstlisting}[language=Python]
% SELECT * FROM ACSIncome
% WHERE working_hours >= 40 and
% Educational_attainment >= 19 and
% Class_of_worker >= 3
% \end{lstlisting} & Erica~\cite{LM23} \\ \cline{2-4}
%   & Q5 & \lstset{aboveskip=0pt, belowskip=0pt}\begin{lstlisting}[language=Python]
% SELECT * FROM ACSIncome
% WHERE working_hours <= 40 and
% Educational_attainment <= 19 and
% Class_of_worker <= 4
% \end{lstlisting} & Generated  \\ \cline{2-4}
%   & Q6 & \lstset{aboveskip=0pt, belowskip=0pt}\begin{lstlisting}[language=Python]
% SELECT * FROM ACSIncome
% WHERE Age >= 35  and
% Class_of_worker >= 2 and
% Educational_attainment <= 15
% \end{lstlisting} & Generated \\ \hline

%          \multirow{2}{*}{TPC-H} & Q7 & \lstset{aboveskip=0pt, belowskip=0pt}\begin{lstlisting}[language=Python]
% SELECT * FROM
% part, supplier, partsupp, nation, region
% WHERE p_partkey = ps_partkey and
% s_suppkey = ps_suppkey
% and s_nationkey = n_nationkey and
% n_regionkey=r_regionkey
% and p_size >= 10 and
% p_type in ('LARGE BRUSHED') and
% r_name in ('EUROPE')
% \end{lstlisting} & Generated inspired by TPC-H's Q2 \\  \hline
%     \end{tabular}
%     }
% \end{table*}

% %%%%%%%%%%%%%%%%%%%%%%%%%%%%%%%%%%%%%

\section{Effect of Solution Exploration Distance}
\captionsetup[figure]{skip=5pt} % Adjust the value as needed

\begin{figure*}[t]
    \centering
    % First row
    \begin{subfigure}[t]{0.49\linewidth}
        \centering
        \includegraphics[width=\linewidth]{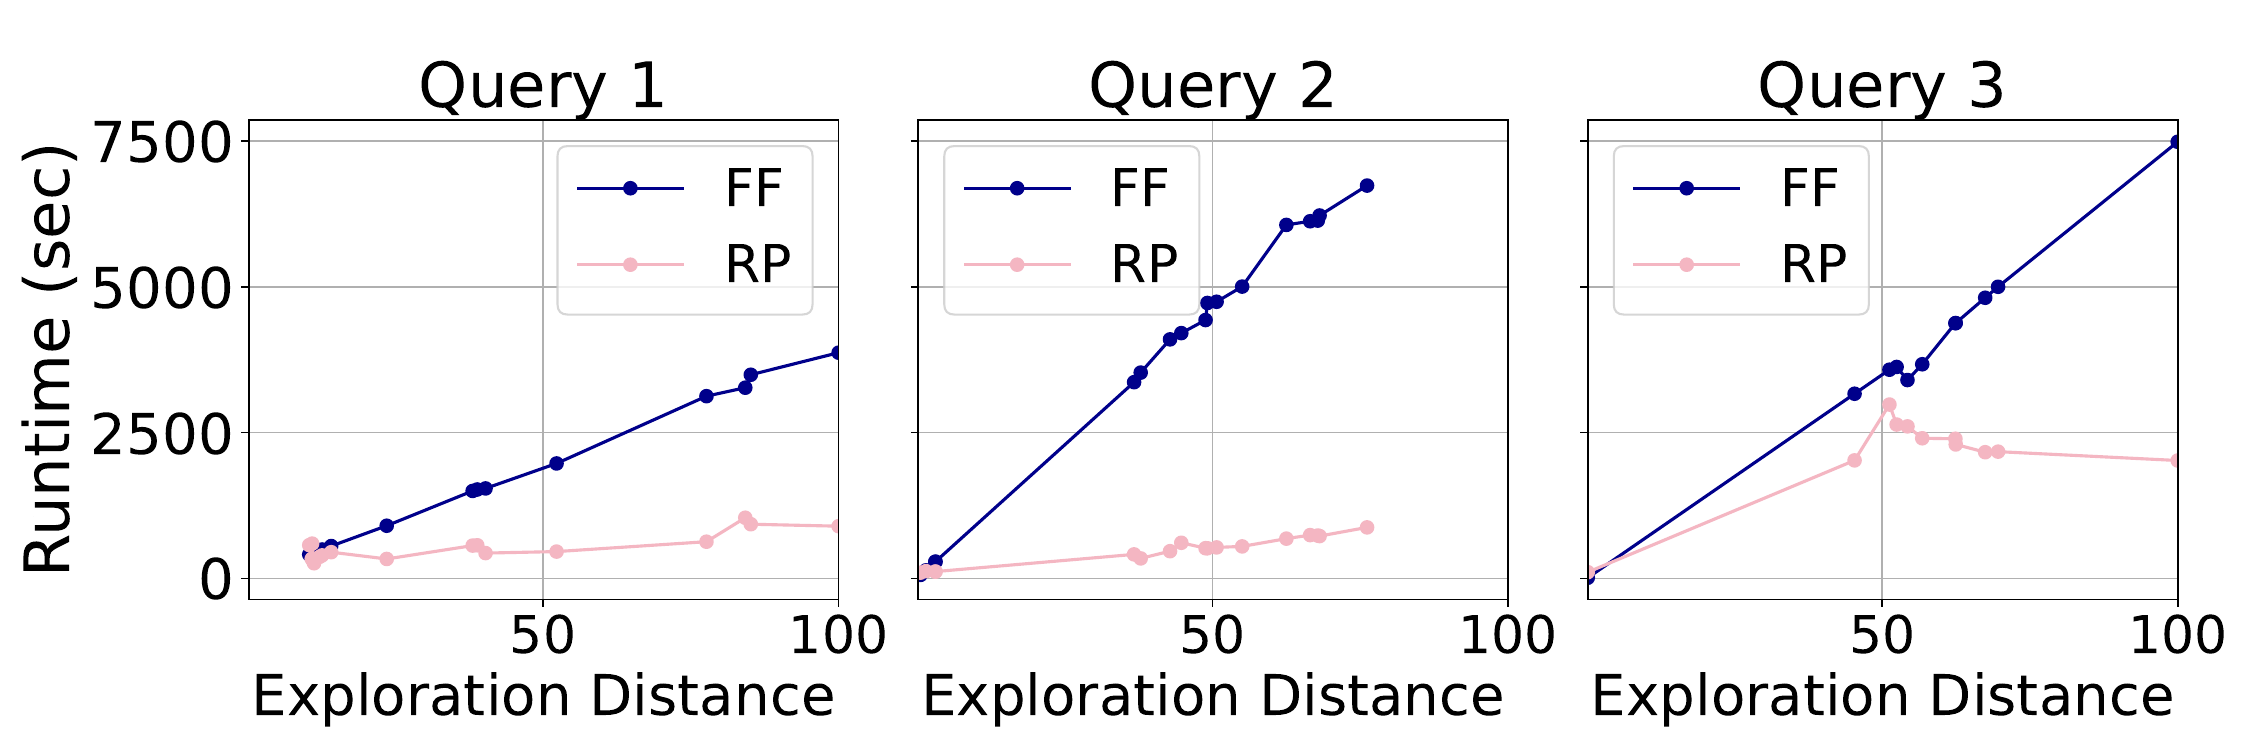}
        \caption{Healthcare dataset.}
        \label{fig:distance_runtime_comparison_healthcare}
    \end{subfigure}
    \hfill
    \begin{subfigure}[t]{0.49\linewidth}
        \centering
        \includegraphics[width=\linewidth]{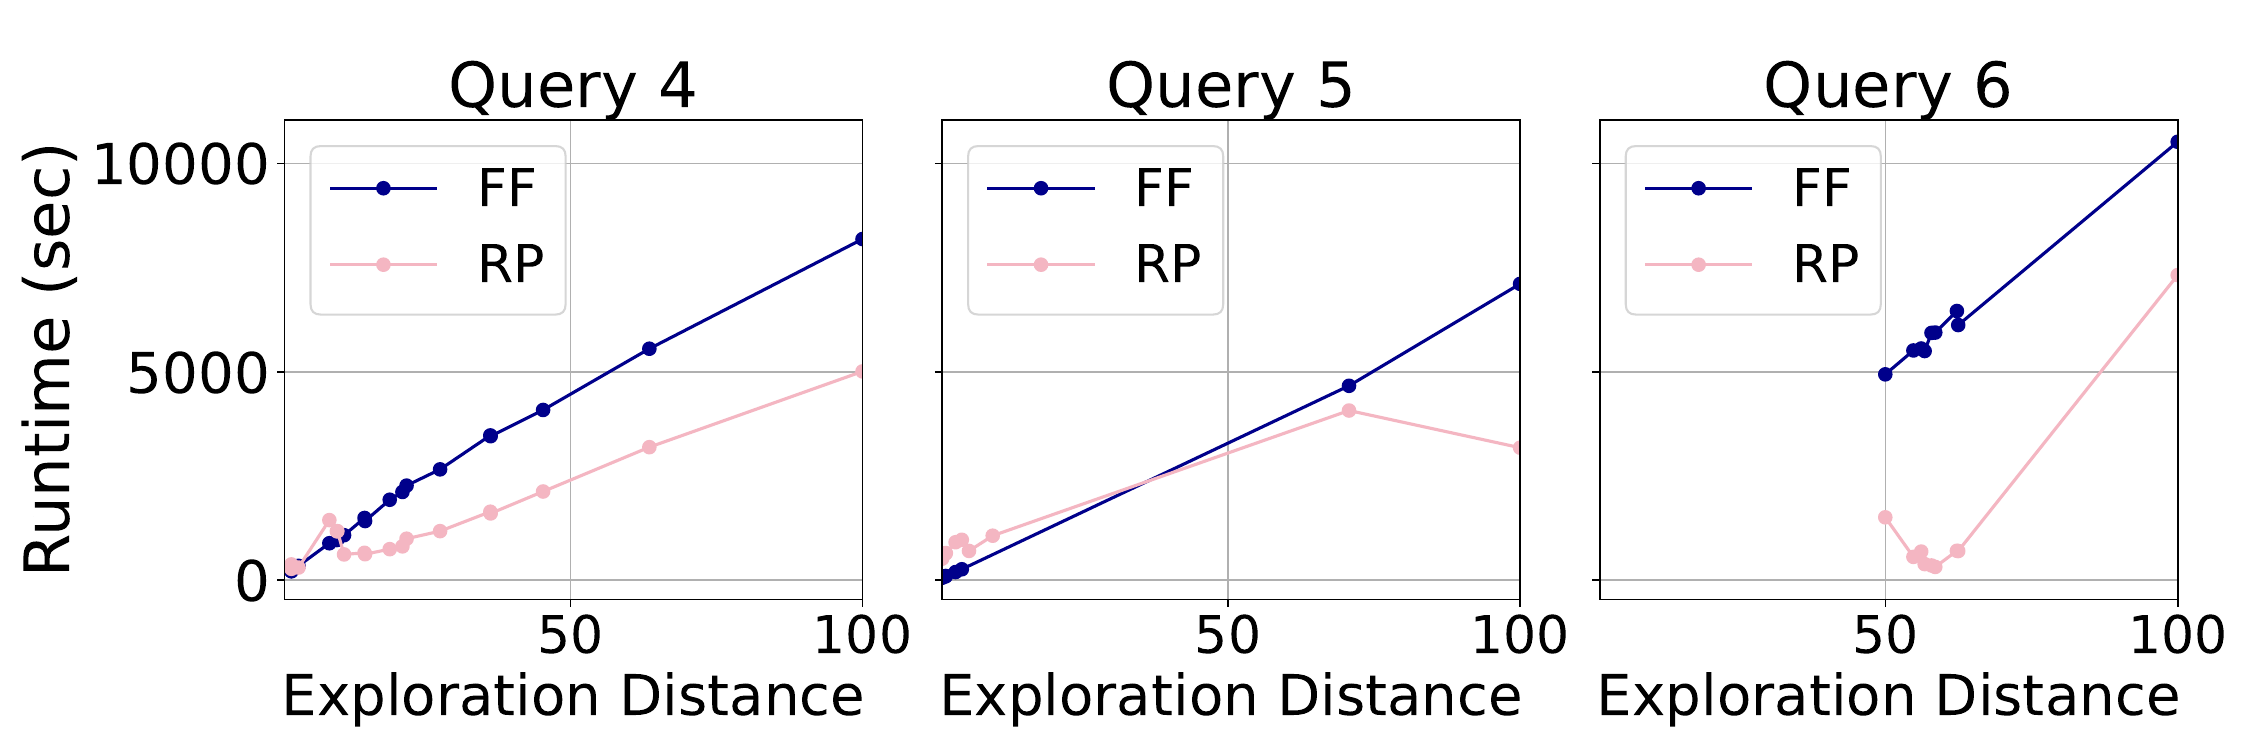}
        \caption{ACSIncome dataset.}
        \label{fig:distance_runtime_comparison_ACSIncome}
    \end{subfigure}
    % Overall caption for the figure
    \caption{Exploration distance comparison of our proposed algorithms.}
    \label{fig:comparison_combined_full}
\end{figure*}
As highlighted in Section \ref{subsec: compare proposed techniques}, constraints with solutions located farther in the search space favor the RP technique, while those closer to the beginning may reduce its advantage. We investigate the impact of solution distance on our proposed algorithms by running queries Q1–Q3 with constraint C1 on the Healthcare dataset using different bounds, and queries Q4–Q6 with constraint C1 on the ACSIncome dataset under varying bounds.

In the Healthcare dataset, we observe same trends across all three measures (Runtime, Candidate solutions checked and Clusters accessed) as Figure \ref{fig:distance_runtime_comparison_healthcare}; therefore, we do not present them here. For Query 1, when the distance is approximately 10\% and less, FF and RP exhibit comparable performance. Similarly, in Queries 2 and 3, when the distance is between 0\% and 3\%, both algorithms perform similarly. However, as the distance increases, we observe a clear advantage for RP, the performance gap widens, indicating that the RP becomes increasingly efficient compared to Fully Filtering Repair. This confirms our previous claim that the RP benefits more when solutions are located farther in the search space.

Similarly, in the ACSIncome dataset, the trends across all three measures as Figure \ref{fig:distance_runtime_comparison_ACSIncome}. For Queries 4 and 5, when the distance is less than 10\%, FF consistently outperforms RP. However, as the distance surpasses 10\%, the performance dynamics shift, favoring RP. This change is reflected by a noticeable reduction in the number of clusters accessed and a decrease in runtime, illustrating that RP becomes increasingly effective as the search space expands.

The reason behind these trends is that when solutions are closer to the start of the search space, FF requires fewer explorations, allowing it to quickly locate a solution that satisfies the constraint. Conversely, RP must examine multiple ranges from the beginning of the search space, leading to increased execution time. These observations reinforce the assertion that the efficiency of the RP repair technique improves as the exploration distance increases, while FF maintains an advantage in scenarios where solutions are in closer proximity.
